# Supplementary material for: Improving \textit{Tug-of-War} sketch using Control-Variates method
Source: arXiv:2203.02432 source file (2022-03-04)
Supplement: Supplementary file 1 [file appendix_plots.tex]

\section{Rough work}
\textcolor{red}{
\begin{align}
\text{Reduced variance}&=\sum_{i\neq j}{f_i}^2{f_j}^2-2\F_2.\\
&=\sum_{i\neq j}{f_i}^2{f_j}^2-2\sum_{i}{f_i}^2.
\end{align}
\begin{align}
\text{Reduced variance}&=\sum_{i\neq j}{f_i}^2{g_j}^2-\frac{2\left(\langle \mathbf{f}, \mathbf{g} \rangle(\F_2+\G_2)\right)^2}{2\langle \mathbf{f}, \mathbf{g} \rangle^2+{\F_2}^2+{\G_2}^2}.
\end{align}
}
\textcolor{blue}{
\begin{align}
    \Cov(X, Z)&=\Cov\left(\sum_{j\in[n]}{f_j}^2 +\sum_{i\neq j,i,j\in[n]}{f_i}{f_j}{Y_i}{Y_j}, \sum_{l\neq m,l,m\in[n]}{Y_l}{Y_m}\right). \numberthis\label{eq:eq200}\\
    &=\Cov\left(\sum_{i\neq j,i,j\in[n]}{f_i}{f_j}{Y_i}{Y_j}, \sum_{l\neq m,l,m\in[n]}{Y_l}{Y_m}\right).\\
    &=\E\left[\left(\sum_{i\neq j,i,j\in[n]}{f_i}{f_j}{Y_i}{Y_j}\right)\cdot\left(\sum_{l\neq m,l,m\in[n]}{Y_l}{Y_m}\right)\right]-\E\left[\sum_{i\neq j,i,j\in[n]}{f_i}{f_j}{Y_i}{Y_j}\right]\cdot\E\left[\sum_{l\neq m,l,m\in[n]}{Y_l}{Y_m}\right].\\
    &=\E\left[\left(\sum_{i\neq j,i,j\in[n]}{f_i}{f_j}{Y_i}{Y_j}\right)\cdot\left(\sum_{l\neq m,l,m\in[n]}{Y_l}{Y_m}\right)\right].\\
    &=\E\left[\sum_{i\neq j,i,j\in[n]}{f_i}{f_j}{{Y_i}}^2{{Y_j}}^2+\sum_{i\neq j\neq l\neq m,i,j,l,m\in[n]}{f_i}{f_j}{{Y_i}}{{Y_j}}{{Y_l}}{{Y_m}}\right].\\
     &=\sum_{i\neq j,i,j\in[n]}{f_i}{f_j}\E\left[{{Y_i}}^2{{Y_j}}^2\right]+\sum_{i\neq j\neq l\neq m,i,j,l,m\in[n]}{f_i}{f_j}\E\left[{{Y_i}}{{Y_j}}{{Y_l}}{{Y_m}}\right].\\
        &=\sum_{i\neq j,i,j\in[n]}{f_i}{f_j}\E\left[1\right]+\sum_{i\neq j\neq l\neq m,i,j,l,m\in[n]}{f_i}{f_j}\times 0.\\
      % &=\sum_{i\neq j,i,j\in[n]}{f_i}{f_j}\E[{{Y_i}}^2]\E[{{Y_j}}^2]+\sum_{i\neq j\neq l\neq m,i,j,l,m\in[n]}{f_i}{f_j}\E[{{Y_i}}]\E[{{Y_j}}]\E[{{Y_l}}]\E[{{Y_m}}].\\
    %   &=\sum_{i\neq j,i,j\in[n]}{f_i}{f_j}+\sum_{i\neq j\neq l\neq m,i,j,l,m\in[n]}{f_i}{f_j}\times 0.\\
       &=\sum_{i\neq j,i,j\in[n]}{f_i}{f_j}.
\end{align}}

\subsection{ Improving the Matrix Multiplication  via Tug-of-War sketch using control variate trick – Proof of Theorem~\ref{thm:}}

\begin{align*}
    %\Cov[X^{(2)},Z^{(2)}]&=\E[X^{(2)}Z^{(2)}]-\E[X^{(2)}]\E[Z^{(2)}]
    &X^{(2)}Z^{(2)}\\&=\left(\sum_{i=1}^n f_i Y_i \right)\cdot \left(\sum_{i=1}^n g_i Y_i \right)\left[\left(\sum_{i=1}^n f_i Y_i \right)^2+\left(\sum_{i=1}^n g_i Y_i \right)^2 \right].\\
    &=\left[\sum_{i=1}^n {f_i g_i} {Y_i}^2 + \sum_{i\neq j, i, j \in [n]} f_ig_j Y_i Y_j  \right]\\&\times\left[\sum_{i=1}^n {f_i}^2 {Y_i}^2 + \sum_{i\neq j, i, j \in [n]} f_if_j Y_i Y_j +\right\\ &\left+\sum_{i=1}^n {g_i}^2 {Y_i}^2 + \sum_{i\neq j, i, j \in [n]} g_ig_j Y_i Y_j  \right].\\
    &=\left[\sum_{i=1}^n {f_i g_i} + \sum_{i\neq j, i, j \in [n]} f_ig_j Y_i Y_j  \right]\times\\&\times\left[\sum_{i=1}^n {f_i}^2 + \sum_{i\neq j, i, j \in [n]} f_if_j Y_i Y_j +\sum_{i=1}^n {g_i}^2 + \sum_{i\neq j, i, j \in [n]} g_ig_j Y_i Y_j  \right].\\
     &=\left[\sum_{i=1}^n {f_i g_i} + \sum_{i\neq j, i, j \in [n]} f_ig_j Y_i Y_j  \right]\times\\&\times\left[\F_2 + \sum_{i\neq j, i, j \in [n]} f_if_j Y_i Y_j +\G_2 + \sum_{i\neq j, i, j \in [n]} g_ig_j Y_i Y_j  \right].\\
&\E[X^{(2)}Z^{(2)}]=(\F_2+\G_2)\cdot\sum_{i=1}^n {f_i g_i} +\\&+ \sum_{i=1}^n {f_i g_i} \left(\sum_{i\neq j, i, j \in [n]}\E[ g_ig_j Y_i Y_j]+\sum_{i\neq j, i, j \in [n]}\E[ f_if_j Y_i Y_j] \right)+\\
&+(\F_2+\G_2)\cdot \sum_{i\neq j, i, j \in [n]}\E[ f_ig_j Y_i Y_j]+\\&+ \E\left[\sum_{i\neq j, i, j \in [n]} f_ig_j Y_i Y_j \left(\sum_{i\neq j, i, j \in [n]} f_if_j Y_i Y_j+\sum_{i\neq j, i, j \in [n]} g_ig_j Y_i Y_j \right) \right].\\
&=(\F_2+\G_2)\cdot\sum_{i=1}^n {f_i g_i}+\E\left[\sum_{i\neq j, i, j \in [n]} {f_i}^2f_jg_j (Y_i Y_j)^2\right] + \\&+\E\left[\sum_{i\neq j, l\neq m} {f_i}g_jf_lf_m Y_i Y_j Y_l Y_m \right]+\\
&+\E\left[\sum_{i\neq j, i, j \in [n]} {f_i}g_i{g_j}^2 (Y_i Y_j)^2 + \sum_{i\neq j, l\neq m} {f_i}g_jg_lg_m Y_i Y_j Y_l Y_m \right].\\
&=(\F_2+\G_2)\cdot\sum_{i=1}^n {f_i g_i}+\sum_{i\neq j, i, j \in [n]} {f_i}^2f_jg_j+\sum_{i\neq j, i, j \in [n]} {f_i}g_i{g_j}^2. \label{eq:expected_dot_prodcut}
\end{align*}

Thus Equations~\eqref{eq:expected_dot_prodcut}, \eqref{eq:cv_dot_product}, and \eqref{eq:expectation_dot_product2} give us the following:
\begin{align*}
  &\Cov[X^{(2)},Z^{(2)}]=\E[X^{(2)}Z^{(2)}]-\E[X^{(2)}]\E[Z^{(2)}].\\
  &=(\F_2+\G_2)\cdot\sum_{i=1}^n {f_i g_i}+\sum_{i\neq j, i, j \in [n]} {f_i}^2f_jg_j+\sum_{i\neq j, i, j \in [n]} {f_i}g_i{g_j}^2- (\F_2+\G_2)\cdot\sum_{i=1}^n {f_i g_i}.\\
  &=\sum_{i\neq j, i, j \in [n]} {f_i}^2f_jg_j+\sum_{i\neq j, i, j \in [n]} {f_i}g_i{g_j}^2.\label{eq:cov_dot_prodcut}
\end{align*}

We now compute the variance of our control variate random variable $Z^{(2)}$ as follows. 
\begin{align}
  {Z^{(2)}}&= (\Tilde{f}^2+\Tilde{g}^2)= \left(\sum_{i=1}^n f_i Y_i \right)^2+\left(\sum_{i=1}^n g_i Y_i \right)^2  .\\
  &= \sum_{i=1}^n {f_i}^2 {Y_i}^2+\sum_{i\neq j}^n {f_i f_j} {Y_iY_j} +\sum_{i=1}^n {g_i}^2 {Y_i}^2+\sum_{i\neq j}^n {g_i g_j} {Y_iY_j}.\\
  &= \F_2+ \G_2+\sum_{i\neq j}^n {f_i f_j} {Y_iY_j} +\sum_{i\neq j}^n {g_i g_j} {Y_iY_j}.\\
  \Var[{Z^{(2)}}]&=\Var\left[\F_2+ \G_2+\sum_{i\neq j}^n {f_i f_j} {Y_iY_j} +\sum_{i\neq j}^n {g_i g_j} {Y_iY_j} \right].\\
  &=\Var\left[ \sum_{i\neq j}^n {f_i f_j} {Y_iY_j} +\sum_{i\neq j}^n {g_i g_j} {Y_iY_j} \right].\\
  &=\E\left[ \left(\sum_{i\neq j}^n {f_i f_j} {Y_iY_j} +\sum_{i\neq j}^n {g_i g_j} {Y_iY_j} \right)^2 \right]-\E\left[\sum_{i\neq j}^n {f_i f_j} {Y_iY_j} +\sum_{i\neq j}^n {g_i g_j} {Y_iY_j}  \right]^2.\\
  &=\E\left[ \left(\sum_{i\neq j}^n {f_i f_j} {Y_iY_j} +\sum_{i\neq j}^n {g_i g_j} {Y_iY_j} \right)^2 \right].\\
  &=\E\left[ \left(\sum_{i\neq j}^n {f_i f_j} {Y_iY_j}\right)^2 +\left(\sum_{i\neq j}^n {g_i g_j} {Y_iY_j} \right)^2+2\left(\sum_{i\neq j}^n {f_i f_j} {Y_iY_j}\right)\left(\sum_{i\neq j}^n {g_i g_j} {Y_iY_j}\right) \right].\\
  &=\E\left[ \sum_{i\neq j}^n {f_i}^2{ f_j}^2 {Y_i}^2{Y_j}^2+\sum_{i\neq j, l\neq m}^n {f_i}{ f_j}{f_l}{ f_m} {Y_i}{Y_j}{Y_l}{Y_m}  \right]+\\&+\E\left[ \sum_{i\neq j}^n {g_i}^2{ g_j}^2 {Y_i}^2{Y_j}^2+\sum_{i\neq j, l\neq m}^n {g_i}{ g_j}{g_l}{ g_m} {Y_i}{Y_j}{Y_l}{Y_m}  \right]+\\+&2\cdot\E\left[\sum_{i\neq j}^n {f_i f_j}{g_i g_j} {Y_i}^2{Y_j}^2+\sum_{i\neq j, l\neq m}^n {f_i f_j}{g_l g_m} {Y_iY_j}{Y_lY_m}\right].\\
  &=\sum_{i\neq j}^n {f_i}^2 {f_j}^2+\sum_{i\neq j}^n {g_i}^2 {g_j}^2+2\sum_{i\neq j}^n {f_ig_i} {f_jg_j}.\label{eq:var_dot_product}
\end{align}
Equations~\eqref{eq:cov_dot_prodcut} and \eqref{eq:var_dot_product} gives us control variate coefficient and variance reduction as follows:
\begin{align}
    \hat{c}&=-\frac{\Cov[X^{(2)},Z^{(2)}]}{\Var[{Z^{(2)}}]}=-\frac{\sum_{i\neq j, i, j \in [n]} {f_i}^2f_jg_j+\sum_{i\neq j, i, j \in [n]} {f_i}g_i{g_j}^2}{\sum_{i\neq j}^n {f_i}^2 {f_j}^2+\sum_{i\neq j}^n {g_i}^2 {g_j}^2+2\sum_{i\neq j}^n {f_ig_i} {f_jg_j}}.\\
    \text{Variance reduction}&=\frac{\Cov[X^{(2)},Z^{(2)}]^2}{\Var[{Z^{(2)}}]}=\frac{\left(\sum_{i\neq j, i, j \in [n]} {f_i}^2f_jg_j+\sum_{i\neq j, i, j \in [n]} {f_i}g_i{g_j}^2\right)^2}{\sum_{i\neq j}^n {f_i}^2 {f_j}^2+\sum_{i\neq j}^n {g_i}^2 {g_j}^2+2\sum_{i\neq j}^n {f_ig_i} {f_jg_j}}.
\end{align}
